# Supplementary material for: Toward Third-Party Assurance of AI Systems: Design Requirements, Prototype, and Early Testing
Source: arXiv:2601.22424 source file (2026-06-01)
Supplement: Supplementary file 1 [file assurance-report-format.pdf]

# AI Assurance Report

## Purpose of this Assurance

The purpose of this Assurance Report is to provide our opinion on the review conducted of <AI system> to determine if 1) the processes (both organizational and technological) by which the AI system is designed, developed, deployed, and monitored for compliance with responsible AI standards, and best practices, and 2) the outputs and outcomes produced as a part of this process are compliant with the intended goals of the system.

## Scope of the Assurance Process

We reviewed the <AI system> from <organization> as of <date>. We interviewed the following individuals: <list of individuals and their corresponding stakeholder roles>. We reviewed the following artifacts: <list of artifacts>.

The interviewees were responsible for providing us with information about the processes used in developing the AI system and the decisions made during those processes. The organization was also responsible for providing us with any related artifacts such as source code for the system (if applicable), any data used to develop and validate the system, and documentation created during these processes, as well as models, analysis results, and related artifacts.

Our responsibility was to conduct this assessment through the interviews and reviewing artifacts provided to us, and provide an opinion as to whether the processes used meet best practices and any standards, and whether the system outputs and the resulting outcomes match the intended function of the AI system.

## Opinion on the AI System

In our opinion, based on the information provided to us, we rate <AI system> overall as follows: <assurance rating>.

In our opinion, we rate each stage of the AI lifecycle for <AI system> as follows.

- Value Proposition + Problem Formulation: <assurance rating>.
- Data Collection + Processing: <assurance rating>.
- Statistical Modeling: <assurance rating>.
- Testing + Validation: <assurance rating>.
- Deployment + Monitoring: <assurance rating>.

## Assurance Ratings

We provide one of the four assurance ratings for the AI system overall, and for each stage.

- 1: Inadequate access to perform the evaluation.
- 2: Adequate access, lack of compliance with baseline industry expectations.
- 3: Adequate access; adequate compliance with baseline expert expectations but lack of evidence of compliance with state of the art and best practices.
- 4: Adequate access, adequate compliance with best practices, and state of the art industry standards.

# Basis for Opinion

<AI system> is the responsibility of <organization>. Our responsibility is to express an opinion on <organization>'s <AI system> based on our assurance process. We are <assurance team> and are required to be independent with respect to <organization>.

We conducted the assurance process by interviewing the representatives from <list of stakeholder roles> using the interview protocol and reviewing <list of artifacts>. Using the interviews, we filled out the "process" column of the maturity matrix; using the artifacts, we filled out the "outputs" column of the maturity matrix. Figure 1 summarizes the ratings we provided for each subcategory in the maturity matrix.

1 - Lagging
2 - Basic
3 - Intermediate
4 - Industry Leading

| Value Proposition + Problem Formulation | | Data Collection + Processing | | Statistical Modeling | | Testing + Validation | | Deployment + Monitoring | |
|---|---|---|---|---|---|---|---|---|---|
| Process | Outputs | Process | Outputs | Process | Outputs | Process | Outputs | Process | Outputs |
| Purpose, Goals, Motivation | Purpose, Goals, Motivation | Data Needs and Requirements | Data Needs and Requirements | Experimental Set Up | Experimental Set Up | Experimental Design | Experimental Design | End User Guidance | End User Guidance |
| Technical Feasibility | Technical Feasibility | Data Availability | Data Availability | Data Set Up | Data Set Up | Considering Alternatives | Considering Alternatives | Use Case Guidance | Use Case Guidance |
| Organizational Feasibility | Organizational Feasibility | Data Collection | Data Collection | Model Choices | Model Choices | Conclusions | Conclusions | System Transparency | System Transparency |
| Risks, Harms, Mitigations | Risks, Harms, Mitigations | Data Lifecycle | Data Lifecycle | Match to Deployment Context | Match to Deployment Context | Impact Assessment | Impact Assessment | Regulatory Compliance | Regulatory Compliance |
| Considering Alternatives | Considering Alternatives | Data Sharing | Data Sharing | Requirement Satisfaction | Requirement Satisfaction | Stakeholder Engagement | Stakeholder Engagement | Governance and Audit Trails | Governance and Audit Trails |
| External Impact Assessment | External Impact Assessment | Legal and Ethical Compliance | Legal and Ethical Compliance | Stakeholder Engagement | Stakeholder Engagement | Process Documentation | Process Documentation | Monitoring | Monitoring |

| | | | | | | | | | |
|---|---|---|---|---|---|---|---|---|---|
| Problem Formulation | Problem Formulation | Preprocessing and Cleaning | Preprocessing and Cleaning | Process Documentation | Process Documentation | | | Maintenance and Updates | Maintenance and Updates |
| Stakeholder Engagement | Stakeholder Engagement | Stakeholder Engagement | Stakeholder Engagement | | | | | Risk Management, Harm Prevention | Risk Management, Harm Prevention |
| Process Documentation | Process Documentation | Process Documentation | Process Documentation | | | | | Stakeholder Engagement | Stakeholder Engagement |
| | | | | | | | | Process Documentation | Process Documentation |

Figure 1: Summary of the maturity matrix that will be included in the final AI Assurance Report. Each column represents a different stage of the AI lifecycle. Each row represents one of the subcategories for that stage. The colors represent the rating that was assigned to that subcategory.

# Recommendations

We recommend the following steps. For <list of subcategories with a subcategory rating of 1 - Lagging>, we recommend that <steps needed to move to 2 - Basic, using the language from the maturity matrix>. For <list of subcategories with a subcategory rating of 2 - Basic>, we recommend that <steps needed to move to 3 - Intermediate, using the language from the maturity matrix>.
