# Supplementary material for: Toward Third-Party Assurance of AI Systems: Design Requirements, Prototype, and Early Testing
Source: arXiv:2601.22424 source file (2026-06-01)
Supplement: Supplementary file 2 [file maturity-matrix.pdf]

# Value Proposition and Problem Formulation

| Process | | | | | Outcomes | | | | |
|---|---|---|---|---|---|---|---|---|---|
| **Category** | **1 - Lagging** | **2 - Basic** | **3 - Intermediate** | **4 - Industry Leading** | **Category** | **1 - Lagging** | **2 - Basic** | **3 - Intermediate** | **4 - Industry Leading** |
| Purpose, Goals, Motivation<br><br>There is a sound process for defining the purpose, goals, and motivations of the AI system by identifying the problem, use cases, and goals, while considering potential harms and impacts. | The team has not considered the business purpose, goals, and motivation behind the AI system. | The team has considered the purposes, goals, and motivations behind the AI system.<br><br>However, the team has not considered one of the following: the primary intended use case is, who the primary intended users are. | The team has considered the purposes, concrete and measurable goals, and motivations behind the AI system.<br><br>This includes what the primary intended use case is and who the primary intended users are.<br><br>They have not prioritized the goals or considered tradeoffs across the goals | The team has thoroughly considered the purpose, goals, and motivation behind the AI system.<br><br>This includes what the primary intended use case is, who the primary intended users are, and enumerated a set of prioritized goals for the system to achieve.<br><br>Additional notes: What problem is it solving?<br><br>Who is it solving it for?<br><br>How much better (in multiple dimensions) does it need to be in order to be used | Purpose, Goals, Motivation<br><br>The AI system's purpose, goals, and motivations point to a realistic net benefit. The goals align with the business need.<br><br>Is there a realistic net benefit to the AI system? | There is no clear purpose, measurable goal, or motivation behind the AI system. | There is a somewhat reasonable and plausible purpose, goal, or motivation for the AI system.<br><br>Additional notes: on the surface, it seems reasonable, but it may be easy to poke holes at it. | There is a reasonable and plausible net-benefit for the AI system and measurable and concrete goals.<br><br>Additional notes: the value proposition seems reasonable and it seems fair enough that the AI system (as envisioned) would bring a net-benefit. It might not be realistic to achieve in practice though. | There is a reasonable and plausible net-benefit for the AI system. It is realistic to assume that the net-benefit will be realized in practice. There is a set of prioritized goals with tradeoffs considered that match the business need. |
| Technical Feasibility and Internal Capacity<br><br>There is a sound process for assessing the | The team has not considered the computational, software, and people resources required nor the | The team has partially considered the computational and software resources required nor the | The team has considered the computational and software resources required and the costs of | The team has considered the computational and software resources required and the costs of | Technical Feasibility and Internal Capacity<br><br>The project is technically feasible and cost | The project is not technically feasible or cost effective. | The project is technically feasible and cost effective, but there have to be many steps taken to realize | The project is technically feasible and cost effective, but there have to be some steps taken to realize | The project is technically feasible and cost effective. |

| Process | | | | | Outcomes | | | | |
|---|---|---|---|---|---|---|---|---|---|
| **Category** | **1 - Lagging** | **2 - Basic** | **3 - Intermediate** | **4 - Industry Leading** | **Category** | **1 - Lagging** | **2 - Basic** | **3 - Intermediate** | **4 - Industry Leading** |
| computational, software, and people resources required to develop, deploy, and maintain the AI system while addressing uncertainties. | costs of developing, deploying, and maintaining the AI system. | costs of developing, deploying, and maintaining the AI system.<br><br>The team has explored technical feasibility and resources in at least one part of the AI lifecycle (ex. development, deployment, maintenance), but has not done this for all stages of the AI lifecycle. | developing, deploying, and maintaining the AI system.<br><br>There is some room for improvement – the analysis of the technical feasibility and resources has taken into account most but not all uncertainties and unknowns (ex. Uncertainty in the exact amount of compute available, how many people will need to monitor the AI system, etc.). | developing, deploying, and maintaining the AI system. | effective, with all required steps being reasonable and practical to achieve.<br><br>Is the project technically feasible? | | this feasibility (ex. Buying more compute). It is somewhat plausible to assume that these steps can be executed. | this feasibility (ex. Buying more compute). It is reasonable to assume that these steps can be executed. | |
| Organizational Feasibility<br><br>There is a process in place for assessing how the AI system aligns with or requires changes to existing business processes and work flows.<br><br>Does the organization have the people | The team has not considered how the task being solved is accomplished today, and how the AI system will be embedded into existing business processes. | The team has considered how the task being solved is accomplished today.<br><br>The team has taken some steps to understand one aspect (best practices or business model).<br><br>There is room for improvement – for example, by getting | The team has considered and has approval/buy-in to how the AI system will either fit into existing business processes or require a change in business processes.<br><br>There is some room for improvement – the team has a good understanding of | The team has considered and has approval/buy-in to how the AI system will either fit into existing business processes or require a change in business processes. | Organizational Feasibility<br><br>The AI system aligns with existing company best practices, fits into the business model, and addresses needed workflow changes effectively.<br><br>Does the AI system align with existing best practices and | The status quo is better than the AI system across all the relevant organizational feasibility dimensions. | The AI system aligns with some of the existing best practices and somewhat fits into the business model.<br><br>There are some major changes to workflows as a result of the AI system, and considering these changes, the AI system does not fit in | The AI system aligns with most of the existing best practices and mostly fits into the business model.<br><br>There are some major changes to workflows as a result of the AI system, but considering these changes, overall, the AI system still fits | The AI system aligns with existing best practices and fits into the business model. |

| Process | | | | | Outcomes | | | | |
|---|---|---|---|---|---|---|---|---|---|
| **Category** | **1 - Lagging** | **2 - Basic** | **3 - Intermediate** | **4 - Industry Leading** | **Category** | **1 - Lagging** | **2 - Basic** | **3 - Intermediate** | **4 - Industry Leading** |
| and organizational structure to incorporate the AI system into the workflow of the larger business process it is supporting? | | approval/buy-in to how the AI system will either fit into existing business processes or require a change in business processes. | existing business processes, but this knowledge could be further supplemented by asking additional people or consulting more existing documentation, for example. | | organizational workflows? | | well with the business model. | into the business model. | |
| Risks, Harms, and Mitigations<br><br>There is a process for identifying risks and harms of using the AI system, and has a process for developing mitigation strategies.<br><br>Additional notes: this is more about risks and harms in how the model can be used. "Impact Assessment" is more about the second-, third-order things that can happen when the model is used (in its primary way) | The team has not considered potential risks, harms, or mitigation strategies. | The team has partially considered risks, harms, and mitigations, but significant gaps remain.<br><br>The team has attempted to identify at least one highly impactful and likely harm/risk and has tried to develop a mitigation. | The team has considered all the highly impactful and likely potential risks, harms, and mitigations.<br><br>This includes a consideration of the people that might misuse the AI system and whether the AI system privileges a certain group of people. Additionally, there is a consideration of the primary, secondary, and unintended uses of the AI system. | The team has considered a sufficient number of the potential risks, harms, and mitigations.<br><br>This includes a consideration of the people that might misuse the AI system and whether the AI system privileges a certain group of people. Additionally, there is a consideration of the primary, secondary, and unintended uses of the AI system. | Risks, Harms, and Mitigations<br><br>The AI system addresses potential risks and harms through concrete and comprehensive mitigations (technical and procedural) that are fully detailed and actionable.<br><br>Does the AI system have potential risks and harms? How severe are they? Are there mitigations? How comprehensive are they? | The AI system has many potential risks and harms that are severe and highly likely.<br><br>There are no proposed mitigations. | The AI system has potential risks and harms. For some of the risks and harms, there are mitigations, such as a document for end-users outlining inappropriate uses that could cause harm. However, these mitigations are very broad. Substantial work in specification would have to be done to execute the mitigation process. | The AI system has potential risks and harms. For the most impactful and likely risks and harms, there are mitigations, such as a document for end-users outlining inappropriate uses that could cause harm. These mitigations are relatively concrete and comprehensive. However to execute one, there would need to be some additional specification to the mitigation process. | The AI system has potential risks and harms. For a sufficient number of the risks and harms, there are mitigations (technical and process), such as a document for end-users outlining inappropriate uses that could cause harm. These mitigations are concrete and comprehensive – to execute one, there would not need to be any additional specification to the mitigation process. |
| Considering Alternatives – | The team has not considered the existing | The team has considered the existing | The team has considered the existing | The team has considered a sufficient number | Considering Alternatives – | There is no reason to believe that the AI | There is some reason to believe that the AI | There is strong reason to believe that the AI | There is strong reason to believe that the AI |

| Process | | | | | Outcomes | | | | |
|---|---|---|---|---|---|---|---|---|---|
| **Category** | **1 - Lagging** | **2 - Basic** | **3 - Intermediate** | **4 - Industry Leading** | **Category** | **1 - Lagging** | **2 - Basic** | **3 - Intermediate** | **4 - Industry Leading** |
| Value Proposition<br><br>There is a process for evaluating the existing solution for the problem and exploring alternative solutions in depth. | approach to the problem (if it exists) as a baseline as well as not considered any simpler, non-AI alternatives. | approach to the problem (if it exists) as a baseline. | approach to the problem (if it exists) as a baseline as well as some simple non-AI alternatives but has explored them with limited depth.<br><br>This includes a consideration of how AI contributes in ways other technologies cannot. | of non-AI alternatives and explored them with great depth.<br><br>This includes a consideration of how AI contributes in ways other technologies cannot. | Value Proposition<br><br>There is evidence that the AI system outperforms the status quo and other alternatives across key dimensions.<br><br>Does the AI system outperform the status quo and other alternatives? | system would be better than the status quo across any of the relevant dimensions. | system would be better than the status quo across all key dimensions such as scale, speed, etc. | system would be better than the status quo and some reason to believe that it would be better than simple non-AI alternatives across all key dimensions such as scale, speed, etc. | system would be better than the status quo and other non-AI alternatives across all key dimensions such as scale, speed, etc. |
| External Impact Assessment<br><br>There is a process for assessing social, environmental, cultural, and political impacts of the AI system.<br><br>Additional notes: this considers impact outside of the organization. | The team has not considered the potential impacts outside the organization, including the positive or negative social, environmental, cultural, and political impacts of the project. | The team has identified a few likely impacts (either positive or negative) of the proposed AI system on external stakeholders and contexts, but this analysis is limited in scope.<br><br>The analysis is limited in that it fails to consider one of the following: how the impacts would be distributed, the change in impacts over time, intended and unintended impacts, and | The team has considered the most important potential positive and the negative social, environmental, cultural, and political impacts of the project.<br><br>This includes how the impacts would be distributed, the change in impacts over time, intended and unintended impacts, and how impact can be measured. | The team has considered a sufficient number of the potential positive and the negative social, environmental, cultural, and political impacts of the project.<br><br>This includes how the impacts would be distributed, the change in impacts over time, intended and unintended impacts, and how impact can be measured. | External Impact Assessment<br><br>There is evidence that the positive impacts of the AI system outweigh the negative impacts, while considering distributions of impacts, changes over time, and intended and unintended consequences<br><br>Do the positive impacts of the AI system outweigh the negative? | There is strong evidence that the anticipated positive impacts of the AI system do not outweigh the anticipated negative impacts, but the project moved ahead. | There is some reason to think that anticipated positive impacts of the AI system outweigh the anticipated negative impacts. There is no mitigation plan for the negative impacts. | There is strong evidence that the anticipated positive impacts of the AI system outweigh the anticipated negative impacts. There is no mitigation plan for the negative impacts.<br><br>This is true when taking into consideration most of the following: how the impacts would be distributed, the change in impacts over time, and intended and | There is strong reason to believe that the anticipated positive impacts of the AI system outweigh the anticipated negative impacts. There is a strong mitigation plan for negative impacts.<br><br>This is true when taking into consideration all of the following: how the impacts would be distributed, the change in impacts over time, and intended and |

| Process | | | | | Outcomes | | | | |
|---|---|---|---|---|---|---|---|---|---|
| **Category** | **1 - Lagging** | **2 - Basic** | **3 - Intermediate** | **4 - Industry Leading** | **Category** | **1 - Lagging** | **2 - Basic** | **3 - Intermediate** | **4 - Industry Leading** |
| | | how impact can be measured. | | | | | | unintended impacts. | unintended impacts. |
| Problem Formulation<br><br>There is a process in place for translating the business problem into a technical problem, while exploring the implications of different approaches. | The team has not deliberately considered ways of translating the business problem into a technical problem. | The team has considered a limited number of ways of translating the business problem into a technical problem, but explored them with limited depth.<br><br>There wasn't enough preliminary work done to fully understand the implications of different choices. | The team has considered a sufficient number of ways of translating the business problem into a technical problem, and explored them with some depth.<br><br>The team has explored various problem formulations with some depth, but there wasn't enough preliminary work done to fully understand the implications of different choices. | The team has considered a sufficient number of ways of translating the business problem into a technical problem, and explored them with great depth.<br><br>In particular, there was preliminary work done to understand the implications of different choices before making a decision on problem formulation. | Problem Formulation<br><br>Is the problem formulation good, and supported by evidence? | There is no deliberate system for translating the business problem into a technical problem.(using a lot of default choices that are likely to be wrong and not match the deployment context) | There is a deliberate system for translating the business problem into a technical problem, but it is either unclear or not well-founded.<br><br>Additional notes: There was a deliberate choice for problem formulation made, but the reasons behind the choice are weak. | There is a deliberate, clear, and well-founded system for translating the business problem into a technical problem.<br><br>Additional notes: There was a deliberate choice for problem formulation made, and the reasons behind the choice are fair. However, there hasn't been any preliminary experimentation. | There is a deliberate, clear, and well-founded system for translating the business problem into a technical problem. There are results from preliminary work done to understand the implications of different choices before making a decision on problem formulation. |
| Stakeholder Engagement<br><br>There is a process for engaging all relevant stakeholders, aligning with the RACI matrix, and incorporating feedback. | The team has not engaged any of the relevant stakeholders. | The team has engaged some of the relevant stakeholders and has incorporated some of their feedback. | The team has engaged most of the relevant stakeholders and has meaningfully incorporated most of their useful and valid input and feedback.<br><br>There are feedback mechanisms for most relevant stakeholders to provide their opinion on the | The team has engaged representatives from all of the relevant stakeholder groups. Each stakeholder's involvement aligns with the RACI matrix column for value proposition and problem formulation.<br><br>There are easily accessible | Stakeholder Engagement<br><br>Has stakeholder input been taken into account? | The input from the relevant stakeholders has not been incorporated into the final value proposition and problem formulation. | Some of the input from the relevant stakeholders has not been incorporated into the final value proposition and problem formulation. | Most of the input from the relevant stakeholders has not been incorporated into the final value proposition and problem formulation. | All of the input from the relevant stakeholders has not been incorporated into the final value proposition and problem formulation, in accordance with the ideal RACI matrix column for value proposition and problem formulation. |

| Process | | | | | Outcomes | | | | |
|---|---|---|---|---|---|---|---|---|---|
| **Category** | **1 - Lagging** | **2 - Basic** | **3 - Intermediate** | **4 - Industry Leading** | **Category** | **1 - Lagging** | **2 - Basic** | **3 - Intermediate** | **4 - Industry Leading** |
| | | | value proposition and problem formulation surrounding the AI system as the system moves through the subsequent stages of the lifecycle. | feedback mechanisms for all relevant stakeholders to provide their opinion on the value proposition and problem formulation surrounding the AI system as the system moves through the subsequent stages of the lifecycle. | | | | | |
| Process Documentation<br><br>There is a process for documenting decisions undertaken during this stage. | The team has not documented any of the processes taken in the value proposition and problem formulation stage in a readily accessible manner. | The team has documented some of the processes taken in the value proposition and problem formulation stage in a readily accessible manner. | The team has documented most of the processes taken in the value proposition and problem formulation stage in a readily accessible manner. | The team has documented all of the processes taken in the value proposition and problem formulation stage in a readily accessible manner. | Outcome Documentation<br><br>Have all the outcomes of this stage been documented? | The team has not documented any of the outcomes of the value proposition and problem formulation stage in a readily accessible manner. | The team has documented some of the outcomes of the value proposition and problem formulation stage in a readily accessible manner. | The team has documented most of the outcomes of the value proposition and problem formulation stage in a readily accessible manner. | The team has documented all of the outcomes of the value proposition and problem formulation stage in a readily accessible manner. |

# Data Collection and Processing

| Process | | | | | Outcomes | | | | |
|---|---|---|---|---|---|---|---|---|---|
| **Category** | **1 - Lagging** | **2 - Basic** | **3 - Intermediate** | **4 - Industry Leading** | **Category** | **1 - Lagging** | **2 - Basic** | **3 - Intermediate** | **4 - Industry Leading** |
| Data Needs and Requirements<br><br>There is a process for identifying and justifying the necessary data while anticipating challenges and developing plans to address them. | The team has not deliberately considered what data is needed, for what, and any additional data requirements. | The team has named a few data sources or types needed for the AI system, but the analysis is incomplete.<br><br>Key variables or data attributes may be listed, but without clear rationale for why they're required. No plan exists for handling issues. | The team has deliberately considered what data is needed, for what, and any additional data requirements.<br><br>The team has justified requirements, anticipated the most impactful and likely challenges/issues, and has a tangible plan with actions. | The team has deliberately considered what data is needed, for what, and any additional data requirements.<br><br>The team has justified requirements, anticipated all challenges/issues, has a tangible plan with actions and actors. | Data Needs and Requirements<br><br>Outcomes: list of data sources and information needed for this project<br><br>Are the identified data needs and requirements sufficient to build a good AI system? Are they detailed enough? | The data needs and requirements were not explicitly identified. | The data needs and requirements were identified.<br><br>Some of the following were explicitly identified: the breadth, depth, and time span of the data needed identified.<br><br>The data needs and requirements are sufficient to build a good AI system. | The data needs and requirements were identified.<br><br>Most of the following were explicitly identified: breadth, depth, and time span.<br><br>The data needs and requirements are sufficient to build a good AI system. | The data needs and requirements were identified.<br><br>The breadth, depth, and time span of the data needed were explicitly identified.<br><br>The data needs and requirements are sufficient to build a good AI system. |
| Data Availability and New Data Collection<br><br>There is a process for assessing and exploring the available data sources, and for developing data collection contingencies. | The team has not deliberately considered what data is available and how readily the data can be collected. | The team has identified a few potential data sources but without assessing their accessibility or quality.<br><br>The team has identified the data sources, but there are unknowns about constraints such as completeness, cost, etc. | The team has mapped out which internal and external data sources are accessible, and roughly how to obtain them.<br><br>The team has identified constraints, gaps, and some ways to mitigate issues. | The team has deliberately considered what data is available and how readily the data can be collected.<br><br>The team has identified sources, have obtained estimates for cost, time, etc, tested collection processes/pipelines, and have plans in place for contingencies. | Data Availability and New Data Collection<br><br>Is the data needed for this project readily available / able to be collected? | The data needed is not available or cannot be readily collected. | The data needed is available and can be collected, with some difficulty, within a reasonable cost and time frame. | The data needed is available and can be readily collected within a reasonable cost and time frame. | The data needed is available and can be readily collected within a reasonable cost and time frame.<br><br>There is a collection process / pipeline that has been tested for functionality. There is an implemented system for what to do in case of issues. |

| Process | | | | | Outcomes | | | | |
|---|---|---|---|---|---|---|---|---|---|
| **Category** | **1 - Lagging** | **2 - Basic** | **3 - Intermediate** | **4 - Industry Leading** | **Category** | **1 - Lagging** | **2 - Basic** | **3 - Intermediate** | **4 - Industry Leading** |
| Data Collection Process and Quality Assessment<br><br>([Datasheets for Datasets](Datasheets for Datasets))<br><br>Additional notes; we separate out the collection since a lot of data is already sitting there<br><br>There is a process for evaluating the dataset generation process including motivation, composition, collection process, and compliance considerations, relative to the project goals. | The team has not considered the data generation process, the context in which it was collected, motivation, composition, collection process.<br><br>The team has not considered any compliance requirements, potentially unethical steps, nor how to assess whether the data is “good enough” for the goals outlined in the Value Proposition. | The team considered some but not all of the following elements of the dataset: motivation, composition, collection process.<br><br>The team has considered some but not all compliance requirements, potentially unethical steps, and how to assess whether the data is “good enough” for the goals outlined in the Value Proposition. | The team has considered some but not all of the following elements of the dataset: the motivation, composition, collection process.<br><br>The team has considered all compliance requirements, potentially unethical steps, and how to assess whether the data is “good enough” for the goals outlined in the Value Proposition. | The team has considered all of the following elements of the dataset: the motivation, composition, collection process, and taken steps to mitigate and prevent any negative downstream outcomes.<br><br>The team has considered all compliance requirements, potentially unethical steps, and how to assess whether the data is “good enough” for the goals outlined in the Value Proposition. | Data Collection Process and Quality Assessment<br><br>Was data collected in an appropriate manner? Is the data collected sufficient to build a good AI system? | The data collection process was inappropriate in some way (ex. Did not involve an IRB when an IRB should have been involved). | The data collection process was appropriate.<br><br>The data collection process did not violate any compliance requirements and did not involve unethical steps.<br><br>The data may not be “good enough” to be used for the goals outlined in Value Proposition. The data is missing many of the following qualities: it is not missing any useful information, it is representative of the population at hand, it is not overly noisy, it covers a sufficient timespan, and the data lag is minimal. | The data collection process was appropriate.<br><br>The data collection process did not violate any compliance requirements and did not involve unethical steps.<br><br>The data is “good enough” to be used for the goals outlined in Value Proposition, although it is not ideal. The data has most of the following qualities: it is not missing any useful information, it is representative of the population at hand, it is not overly noisy, it covers a sufficient timespan, and the data lag is minimal. | The data collection process was appropriate.<br><br>The data collection process did not violate any compliance requirements and did not involve unethical steps.<br><br>The data is “good enough” to be used for the goals outlined in Value Proposition: it is not missing any useful information, it is representative of the population at hand, it is not overly noisy, it covers a sufficient timespan, and the data lag is minimal. |
| Data Lifecycle<br><br>There is a process to *define* the roles, responsibilities, | The team has not deliberately considered who will be storing / hosting / maintaining / | The team has outlined responsibilities for one or two tasks in the data lifecycle but the | The team has outlined who is responsible for storing, hosting, maintaining, and updating the | The team has deliberately considered who will be storing / hosting / maintaining / | Data Lifecycle<br><br>Is there an implemented system for | There is no implemented system for storing / hosting / maintaining / updating / | There is an implemented system for storing / hosting / maintaining / updating / | There is an implemented system for storing / hosting / maintaining / updating / | There is an implemented system for storing / hosting / maintaining / updating / |

| Process | | | | | Outcomes | | | | |
|---|---|---|---|---|---|---|---|---|---|
| **Category** | **1 - Lagging** | **2 - Basic** | **3 - Intermediate** | **4 - Industry Leading** | **Category** | **1 - Lagging** | **2 - Basic** | **3 - Intermediate** | **4 - Industry Leading** |
| and timelines for storing, hosting, maintaining, updating, and decommissioning the datasets. | updating / decommissioning the dataset, and how these tasks will be done. | overall plan is incomplete.<br><br>There are no roles/schedules/timelines in place. | dataset, along with a broad timeline. | updating / decommissioning the dataset, and how these tasks will be done, along with a specific timeline. | storing / hosting / etc. the dataset? | decommissioning the dataset, and how these tasks will be done. | decommissioning the dataset, with compliance checks implemented.<br><br>This implemented system includes who will be doing each task, and when. To execute the system, there would need to be a lot of additional specification. | decommissioning the dataset, with compliance checks implemented.<br><br>This implemented system includes who will be doing each task, and when. To execute the system, there would need to be some additional specification. | decommissioning the dataset, with compliance checks implemented.<br><br>This implemented system includes who will be doing each task, and when. To execute the system, there would not need to be any additional specification. |
| Data Sharing and Distribution<br><br>There is a process for defining the policies, controls, and terms for sharing data. | The team has not deliberately considered whether data will be made accessible to others, to what extent, and the appropriate terms of use, licensing, and potential uses.<br><br>In addition, no standard organizational defaults exist.<br><br>Additional notes: Default choice of making everything super private. If there is already a default of no sharing, etc. | The team has noted that data might be shared externally or internally but hasn't defined clear policies.<br><br>Possible recipients or platforms may be listed, but without details or specifics. | The team has defined who can access the data, under what conditions, and with basic licensing or terms of use.<br><br>Technical and contractual controls and processes are in place for granting and restricting access. | The team has deliberately considered whether data will be made accessible to others, to what extent, and the appropriate terms of use, licensing, and potential uses. | Data Sharing and Distribution<br><br>Is there a system for making the data accessible to others, etc.? | There is no deliberate implemented system for whether data will be made accessible to others, to what extent, and the appropriate terms of use, licensing, and potential uses.<br><br>Or, there is a deliberate implemented system, but the system is fundamentally flawed in a major way (ex. Violates the privacy of individuals in the dataset). | There is an implemented system for one of the following: making the data accessible to others, to what extent, and the appropriate terms of use, licensing, potential uses.<br><br>The implemented system adheres to existing guidelines (ex. Ethical guidelines). | There is an implemented system for making the data accessible to others, to what extent, and the appropriate terms of use, licensing, and potential uses.<br><br>The implemented system adheres to existing guidelines (ex. Ethical guidelines).<br><br>To execute some of the processes in the system (ex. The process of granting data access), there | There is an implemented system for making the data accessible to others, to what extent, and the appropriate terms of use, licensing, and potential uses.<br><br>The implemented system adheres to existing guidelines (ex. Ethical guidelines). |

| Process | | | | | Outcomes | | | | |
|---|---|---|---|---|---|---|---|---|---|
| **Category** | **1 - Lagging** | **2 - Basic** | **3 - Intermediate** | **4 - Industry Leading** | **Category** | **1 - Lagging** | **2 - Basic** | **3 - Intermediate** | **4 - Industry Leading** |
| | Only applicable if you were the primary data source / data collector / data buyer. Everything is critical if it isn't critical | | | | | | | would need to be some additional specification. | |
| Legal and Ethical Compliance<br><br>Additional notes: This includes security, privacy, etc.<br><br>There is a process for assessing the legal requirements and ethical standards for data use, as well as data subject rights and privacy. | The team has not deliberately considered whether data use is legally and ethically justified, what requirements apply, whether the rights of the data subjects have been respected, nor the implications of or measures to protect data from breaches and unauthorized use. | The team has identified a few relevant laws or ethical guidelines (GDPR, HIPAA) but hasn't fully mapped them to the project's data practices. | The team has deliberately considered whether data use is legally and ethically justified, what requirements apply, and whether the rights of the data subjects have been respected, and the implications of or measures to protect data from the most impactful and likely breaches and unauthorized use. | The team has deliberately considered whether data use is legally and ethically justified, what requirements apply, and whether the rights of the data subjects have been respected, and the implications of or measures to protect data from breaches and unauthorized use. | Legal and Ethical Compliance<br><br>Is the use of data legally and ethically justified? | The use of data is not legally and ethically justified. The applicable requirements are not satisfied. The rights of the data subjects have not been respected. There are no measures to protect data from breaches and unauthorized use. | The use of data is legally and ethically justified. The applicable requirements are satisfied. The rights of the data subjects have been respected. There are measures to protect data from breaches and unauthorized use.<br><br>To execute these measures, there would need to be a lot of additional specification. | The use of data is legally and ethically justified. The applicable requirements are satisfied. The rights of the data subjects have been respected. There are measures to protect data from breaches and unauthorized use.<br><br>To execute these measures, there would need to be some additional specification. | The use of data is legally and ethically justified. The applicable requirements are satisfied. The rights of the data subjects have been respected. There are comprehensive measures to protect data from breaches and unauthorized use. |
| Preprocessing / cleaning<br><br>There is a process for deliberate planning and conducting | The team has not thought about preprocessing, or cleaning the data. | The team has thought about preprocessing, or cleaning the data. However, for many preprocessing / cleaning-related choices, the team cannot | The team has thought about preprocessing or cleaning the data. For most preprocessing / cleaning-related choices, they can articulate why that | The team has thought about preprocessing, cleaning, or labelling the data. For all preprocessing / cleaning-related choices, they can articulate | Data Assessment<br><br>Is the dataset representative of the problem at hand? | The dataset is not representative of the AI problem at hand. The dataset is not representative across all the | The dataset is mostly representative of the AI problem at hand. The dataset is mostly representative across the | The dataset is representative of the AI problem at hand. The dataset is representative across the relevant features and classes. | The dataset is representative of the AI problem at hand. The dataset is representative across the relevant features and classes. |

| Process | | | | | Outcomes | | | | |
|---|---|---|---|---|---|---|---|---|---|
| **Category** | **1 - Lagging** | **2 - Basic** | **3 - Intermediate** | **4 - Industry Leading** | **Category** | **1 - Lagging** | **2 - Basic** | **3 - Intermediate** | **4 - Industry Leading** |
| preprocessing and cleaning. | | articulate why that particular choice was made over alternatives. | particular choice was made over alternatives. | why the particular choice was made over alternatives. | | features and classes. | relevant features and classes.<br><br>To achieve such a dataset, if needed, some of the appropriate preprocessing / cleaning steps have been taken to improve dataset quality, protect confidentiality, and de-identify the dataset. | To achieve such a dataset, if needed, most of the appropriate preprocessing / cleaning steps have been taken to improve dataset quality, protect confidentiality, and de-identify the dataset. | To achieve such a dataset, if needed, all of the appropriate preprocessing / cleaning steps have been taken to improve dataset quality, protect confidentiality, and de-identify the dataset. |
| Stakeholder Engagement<br><br>There is a process for engaging all relevant stakeholders, aligning with the RACI matrix, and incorporating feedback. | The team has not engaged any of the relevant stakeholders. | The team has engaged some of the relevant stakeholders and has incorporated some of their feedback. | The team has engaged most of the relevant stakeholders and has meaningfully incorporated most of their useful and valid input and feedback.<br><br>There are feedback mechanisms for most relevant stakeholders to provide their opinion on the value proposition and problem formulation surrounding the AI system as the system moves through the subsequent stages of the lifecycle. | The team has engaged representatives from all of the relevant stakeholder groups. Each stakeholder's involvement aligns with the RACI matrix column for value proposition and problem formulation.<br><br>There are easily accessible feedback mechanisms for all relevant stakeholders to provide their opinion on the value proposition and problem formulation surrounding the AI system as the system moves | Stakeholder Engagement<br><br>Has stakeholder input been taken into account? | The input from the relevant stakeholders has not been incorporated into the final dataset used. | Some of the input from the relevant stakeholders has not been incorporated into the final dataset used. | Most of the input from the relevant stakeholders has not been incorporated into the final dataset used. | All of the input from the relevant stakeholders has not been incorporated into the final dataset used in accordance with the ideal RACI matrix column for data collection and processing. |

| Process | | | | | Outcomes | | | | |
|---|---|---|---|---|---|---|---|---|---|
| **Category** | **1 - Lagging** | **2 - Basic** | **3 - Intermediate** | **4 - Industry Leading** | **Category** | **1 - Lagging** | **2 - Basic** | **3 - Intermediate** | **4 - Industry Leading** |
| | | | | through the subsequent stages of the lifecycle. | | | | | |
| Process Documentation<br><br>There is a process for documenting decisions undertaken during this stage. | The team has not documented any of the processes taken in the data collection and processing stage in a readily accessible manner. | The team has documented some of the processes taken in the data collection and processing stage in a readily accessible manner. | The team has documented most of the processes taken in the data collection and processing stage in a readily accessible manner. | The team has documented all of the processes taken in the data collection and processing stage in a readily accessible manner. | Outcome Documentation<br><br>Have all the outcomes of this stage been documented? | The team has not documented any of the outcomes of the data collection and processing stage in a readily accessible manner. | The team has documented some of the outcomes of the data collection and processing stage in a readily accessible manner. | The team has documented most of the outcomes of the data collection and processing stage in a readily accessible manner. | The team has documented all of the outcomes of the data collection and processing stage in a readily accessible manner. |

# Statistical Modeling

| Process | | | | | Outcomes | | | | |
|---|---|---|---|---|---|---|---|---|---|
| **Category** | **1 - Lagging** | **2 - Basic** | **3 - Intermediate** | **4 - Industry Leading** | **Category** | **1 - Lagging** | **2 - Basic** | **3 - Intermediate** | **4 - Industry Leading** |
| Modeling Set-Up<br><br>There is a process for defining units of analysis and labels/outcomes so that the experiment aligns with the purpose, goals and motivations. | The team has not considered what each unit of analysis will be (ex. What each row in the dataset represents) or what the labels will be.<br><br>The decisions that the team made in problem formulation do not align with the decisions made in modeling set-up. | The team has considered what each unit of analysis will be (ex. What each row in the dataset represents) and what the labels will be.<br><br>Some, but not all of the decisions that the team made in problem formulation align with the decisions made in modeling set-up. | The team has deliberately considered what each unit of analysis will be (ex. What each row in the dataset represents) and what the labels will be.<br><br>The decisions that the team made in problem formulation align with the decisions made in modeling set-up. | The team has deliberately considered what each unit of analysis will be (ex. What each row in the dataset represents) and what the labels will be.<br><br>The decisions that the team made in problem formulation align with the decisions made in modeling set-up.<br><br>They have explored different labels as proxies for the true label/outcome they care about and settled on the most effective one for the task. | Modeling Set-Up<br><br>Is the modeling set-up appropriate for the problem? | The unit of analysis (ex. What each row in the dataset represents) is not appropriate for the problem. The labels are not appropriate for this problem. | Only one out of the unit of analysis (ex. What each row in the dataset represents) or the labels are appropriate for this problem. | The unit of analysis (ex. What each row in the dataset represents) is appropriate for the problem. The labels are appropriate for this problem.<br><br>There is evidence that discussions on different labels as proxies for the true label/outcome have taken place. | The unit of analysis (ex. What each row in the dataset represents) is appropriate for the problem. The labels are appropriate for this problem.<br><br>There is evidence on different labels as proxies for the true label/outcome, and the evidence empirically shows that the chosen unit of analysis and labels are the most effective for this problem. |
| Features Set-Up<br><br>There is a process for deliberately generating data features and handling missing information. | The team has not deliberately considered what features they are making with the data or how to deal with missing information. | The team has identified a handful of features to extract and noted that missing values exist, but the rationale and | The team has deliberately considered what features they are making with the data and basic methods for how to deal with missing information. For | The team has deliberately considered what features they are making with the data and how to deal with missing information. For each choice, they can explain | Features Set-Up<br><br>Is the features set-up appropriate for the problem? | The features that are used are not appropriate for the problem. The decisions surrounding missing data are not appropriate for the problem. | It is somewhat reasonable to believe that the features that are used are appropriate for the problem. It is somewhat reasonable to believe that the | The features that are used are appropriate for the problem. The decisions surrounding missing data are appropriate for the problem. | The features that are used are appropriate for the problem. The decisions surrounding missing data are appropriate for the problem. |

| Process | | | | | Outcomes | | | | |
|---|---|---|---|---|---|---|---|---|---|
| **Category** | **1 - Lagging** | **2 - Basic** | **3 - Intermediate** | **4 - Industry Leading** | **Category** | **1 - Lagging** | **2 - Basic** | **3 - Intermediate** | **4 - Industry Leading** |
| | | strategy are incomplete. | each choice, they can explain why that choice is a reasonable one. | why that choice was made over others. | | | decisions surrounding missing data are appropriate for the problem.<br><br>There are some additional features that could have been created with the data that could have also been relevant for the problem. | There are some additional features that could have been created with the data that could have also been relevant for the problem. | |
| Models Considered and Used<br><br>There is a process for systematically exploring different model choices, allowing for justified final choices based on model tradeoffs. | The team has not considered multiple types of models. In addition, the team has not deliberately picked the parameters that are needed for their model, and does not know about this. | The team has evaluated a limited selection of model families and run limited initial experiments to compare their performance.<br><br>Some of the choices made throughout this process – such as the parameters to use – fail to consider some key variables (ex. training / inference time, accuracy, fairness, and interpretability). | The team has evaluated a reasonable selection of model families and run initial experiments to compare their performance.<br><br>They have justified their final choice, considering the most relevant tradeoffs for the use case such as training / inference time, accuracy, fairness, and interpretability. | The team has evaluated a sufficient selection of model families and run initial experiments to compare their performance.<br><br>They have justified their final choice, considering tradeoffs such as training / inference time, accuracy, fairness, and interpretability. | Model Considered and Used<br><br>How wide was the set of models considered?<br><br>Additional notes: did the team just try LLMs? Just a decision tree / regression? | No model comparison exists. Just results on one model. | Small set of models were tested and the choice was done in an adhoc manner with no justification. | Small set of models tested but justified through resource and deployment constraints. | Wide variety of models were explored and compared - ranging from simple to complex with a reasonable range of hyperparameters considered for each model type and results across all relevant metrics. |
| Model Selection Methodology – | The team has not considered | The team has given some | The team has considered how | The team has considered how | Model Selection Methodology – | The model selected | The model selected | The model selected mostly | The model selected |

| Process | | | | | Outcomes | | | | |
|---|---|---|---|---|---|---|---|---|---|
| **Category** | **1 - Lagging** | **2 - Basic** | **3 - Intermediate** | **4 - Industry Leading** | **Category** | **1 - Lagging** | **2 - Basic** | **3 - Intermediate** | **4 - Industry Leading** |
| Match to Deployment Context<br><br>There is a process for evaluating model performance that reflects real world conditions. | how different models can generalize to the real-world. | thought to generalization, looking at performance on a held-out test set, but hasn't connected those results to real-world conditions. | different models can generalize to the real-world.<br><br>The team has evaluated models on data splits or simulated conditions that reasonably approximate real-world variability. | different models can generalize to the real-world.<br><br>The team has evaluated models on data splits or simulated conditions that closely approximate real-world variability. | Match to Deployment Context<br><br>Does the chosen model's performance generalize to real-world contexts? | generalizes poorly to the real-world. | generalizes somewhat to the real-world.<br><br>There are key aspects of real-world variability that could likely happen that the model does not generalize to. | generalizes to the real-world.<br><br>There are key aspects of real-world variability that could plausibly happen that the model does not generalize to. | generalizes well to the real-world. |
| Model Selection Methodology – Requirement Satisfaction<br><br>There is a process for defining and evaluating the model against original purpose, goals, and motivations. | The team has not considered model performance metrics and how they align with the goals set in previous stages, such as fairness and privacy requirements. | The team has identified a few performance metrics (accuracy, precision) and noted the high-level goals, but alignment is weak or incomplete. | The team has defined a set of performance metrics that map to earlier goals (ex. selecting both accuracy and a fairness metric).<br><br>They have computed some initial statistics and understand that there are some uncertainties even if they do not have formal metrics for it. | The team has considered model performance metrics and how they align with the goals set in previous stages, such as fairness and privacy requirements.<br><br>For each metric, the team has considered confidence intervals, variability, statistical significance of test results, and uncertainty of the model. | Model Selection Methodology – Requirement Satisfaction<br><br>Does the chosen model meet the goals set in previous stages? | The model performance metrics do not align with the goals set in previous stages, such as fairness and privacy requirements. | The model performance metrics mostly align with the goals set in previous stages, such as fairness and privacy requirements.<br><br>For each metric, some of the following have been recorded: the confidence intervals, variability, statistical significance of test results, and uncertainty of the model. | The model performance metrics aligns with the goals set in previous stages, such as fairness and privacy requirements.<br><br>For each metric, most of the following have been recorded: the confidence intervals, variability, statistical significance of test results, and uncertainty of the model.. | The model performance metrics aligns with the goals set in previous stages, such as fairness and privacy requirements.<br><br>For each metric, the confidence intervals, variability, statistical significance of test results, and uncertainty of the model have been recorded. When these are taken into account, the model performance metrics continue to align with the goals set in previous stages. |

| Process | | | | | Outcomes | | | | |
|---|---|---|---|---|---|---|---|---|---|
| **Category** | **1 - Lagging** | **2 - Basic** | **3 - Intermediate** | **4 - Industry Leading** | **Category** | **1 - Lagging** | **2 - Basic** | **3 - Intermediate** | **4 - Industry Leading** |
| Stakeholder Engagement<br><br>There is a process for engaging all relevant stakeholders, aligning with the RACI matrix, and incorporating feedback. | The team has not engaged any of the relevant stakeholders. | The team has engaged some of the relevant stakeholders and has incorporated some of their feedback. | The team has engaged most of the relevant stakeholders and has meaningfully incorporated most of their useful and valid input and feedback.<br><br>There are feedback mechanisms for most relevant stakeholders to provide their opinion on the value proposition and problem formulation surrounding the AI system as the system moves through the subsequent stages of the lifecycle. | The team has engaged representatives from all the stakeholder groups. Each stakeholder's involvement aligns with the RACI matrix column for value proposition and problem formulation.<br><br>There are easily accessible feedback mechanisms for all relevant stakeholders to provide their opinion on the value proposition and problem formulation surrounding the AI system as the system moves through the subsequent stages of the lifecycle. | Stakeholder Engagement<br><br>Has stakeholder input been taken into account? | The input from the relevant stakeholders has not been incorporated into the final decisions in statistical modeling. | Some of the input from the relevant stakeholders has not been incorporated into the final decisions in statistical modeling. | Most of the input from the relevant stakeholders has not been incorporated into the final decisions in statistical modeling. | All of the input from the relevant stakeholders has not been incorporated into the final decisions in statistical modeling in accordance with the ideal RACI matrix column for statistical modeling. |
| Process Documentation<br><br>There is a process for documenting decisions undertaken during this stage. | The team has not documented any of the processes taken in the statistical modeling stage in a readily accessible manner.<br><br>There is no documentation on the processes taken to decide | The team has documented some of the processes taken in the statistical modeling stage in a readily accessible manner. | The team has documented most of the processes taken in the statistical modeling stage in a readily accessible manner. | The team has documented all of the processes taken in the statistical modeling stage in a readily accessible manner.<br><br>There is documentation on the processes taken to decide | Outcome Documentation<br><br>Have all the outcomes of this stage been documented? | The team has not documented any of the outcomes of the statistical modeling stage in a readily accessible manner.<br><br>There is no documentation on the task, output, | The team has documented some of the outcomes of the statistical modeling stage in a readily accessible manner. | The team has documented most of the outcomes of the statistical modeling stage in a readily accessible manner. | The team has documented all of the outcomes of the statistical modeling stage in a readily accessible manner.<br><br>There is documentation on the task, output, architecture, |

| Process | | | | | Outcomes | | | | |
|---|---|---|---|---|---|---|---|---|---|
| **Category** | **1 - Lagging** | **2 - Basic** | **3 - Intermediate** | **4 - Industry Leading** | **Category** | **1 - Lagging** | **2 - Basic** | **3 - Intermediate** | **4 - Industry Leading** |
| | the task, output, architecture, code, and who and when the model was developed. | | | the task, output, architecture, code, and who and when the model was developed. | | architecture, code, and who and when the model was developed. | | | code, and who and when the model was developed. |

# Testing and Validation

| Process | | | | | Outcomes | | | | |
|---|---|---|---|---|---|---|---|---|---|
| **Category** | **1 - Lagging** | **2 - Basic** | **3 - Intermediate** | **4 - Industry Leading** | **Category** | **1 - Lagging** | **2 - Basic** | **3 - Intermediate** | **4 - Industry Leading** |
| Experimental Design<br><br>There is a process for designing experiments to test the AI system in real world conditions. | The team has not deliberately considered the experimental design for real-world testing.<br><br>The team has not considered what metrics to evaluate the AI system on.<br><br>Additional notes: by testing, it is implied that we are not just testing the model, we are also testing what the end-users are doing and how they are using the model | The team has discussed the experimental design. The discussions have included consideration on some but not all of the important aspects of strong experimental design (appropriate sample size, the methodology, statistical power, and significance).<br><br>The team has considered what metrics to evaluate the AI system on, but not all aspects of how the metrics are relevant to the real-world context in which the model will be used. | The team has discussed the experimental design. The discussions have included consideration on most but not all of the important aspects of strong experimental design (appropriate sample size, the methodology, statistical power, and significance).<br><br>The team has considered what metrics to evaluate the AI system on, and how they are relevant to the real-world context in which the model will be used. | The team has discussed the experimental design. The discussions have included consideration on appropriate sample size, the methodology, statistical power, and significance.<br><br>The team has considered what metrics to evaluate the AI system on, and how they are relevant to the real-world context in which the model will be used. | Experimental Design<br><br>Is there a good experimental design for real-world testing? | There is no deliberate experimental design for real-world testing.<br><br>The metrics chosen to evaluate the AI system are not relevant to the real-world context in which the model will be used. | There is a basic plan for experiments, but it is not comprehensive.<br><br>Methodology details are only loosely defined. | There is a structured, real world experiment with defined processes and populations.<br><br>Sample size is based on power calculations.<br><br>There is a basic methodology in place.<br><br>Evaluation metrics are relevant to the real world deployment.<br><br>Model updates are reactive, based on observed model drift or other factors. | There is a comprehensive experimental design for real-world testing. The experimental design consists of an appropriate sample size and a sound methodology, such that the statistical power and significance of any results from the real-world testing are sufficiently high.<br><br>The metrics chosen to evaluate the AI system are relevant to the real-world context in which the model will be used. There is an assessment on how often the AI system would need to be updated. |
| Alternatives<br><br>There is a process for testing different alternatives, including the | The team has not considered any alternatives in testing. | The team has considered the status quo in testing. | The team has considered alternatives in testing.<br><br>The alternatives include the | The team has considered alternatives in testing.<br><br>The alternatives include the | Alternatives<br><br>Does the AI system outperform the status quo and | There is no reason to believe that the AI system would be better than the status quo | There is some reason to believe that the AI system would be better than the status quo | There is strong reason to believe that the AI system would be better than the status quo and | There is strong reason to believe that the AI system would be better than the status quo and |

| Process | | | | | Outcomes | | | | |
|---|---|---|---|---|---|---|---|---|---|
| **Category** | **1 - Lagging** | **2 - Basic** | **3 - Intermediate** | **4 - Industry Leading** | **Category** | **1 - Lagging** | **2 - Basic** | **3 - Intermediate** | **4 - Industry Leading** |
| status quo, to evaluate the AI system effectively.<br><br>Additional notes: don't have a corresponding "Outcomes" for this, since we didn't have anything for Value Proposition | | | status quo, but not all of the different candidate models from statistical modeling.<br><br>Additional notes: by doing this, the team could build a reasonably good AI system, even if there are other candidate models from Statistical Modeling that could have been better | status quo and different candidate models from statistical modeling. | other alternatives? | across any of the relevant dimensions. | across all key dimensions such as scale, speed, etc. | some reason to believe that it would be better than simple non-AI alternatives across all key dimensions such as scale, speed, etc. | other non-AI alternatives across all key dimensions such as scale, speed, etc. |
| Conclusions<br><br>Additional notes: this is more about the primary goal of the system, while impact assessment is about secondary effects as well.<br><br>There is a process for drawing conclusions that the AI system meets/does not meet the primary goals compared against alternatives. | The team has not done testing that allows the team to conclude that the intended goals of the system have been measured. | The team has done testing that allows the team to analyze the results of each alternative.<br><br>The testing does not fully demonstrate that the intended goals of the system have been measured, but the connection between the testing procedure and the intended goals of the system is plausible. | The team has done testing that allows the team to analyze the results of each alternative and demonstrate that the intended goals of the system have been measured.<br><br>The team is able to make a determination that the AI system has the intended benefits compared to the status quo. | The team has done testing that allows the team to analyze the results of each alternative and demonstrate that the intended goals of the system have been measured.<br><br>The team is able to make a determination that the AI system has the intended benefits compared to the status quo and other alternatives. | Conclusions<br><br>Has the correct alternative been chosen from testing results? | Based on the results of the testing, the correct alternative has not been chosen. | The team reviewed experiment outcomes and compared them against some alternatives, but the selection decision is unclear or incomplete.<br><br>They did not balance multiple metrics and only compared single highest scores. | Based on the results of the testing, the correct alternative has been chosen.<br><br>There is clear documentation for how certain alternatives outperformed others and how the chosen solution meets goals.<br><br>There is reasoning for major trade offs. | Based on the results of the testing, the correct alternative has been chosen.<br><br>There is a rigorous decision making process. All viable solutions were compared across multiple metrics.<br><br>The team considered long term outcomes like maintainability or scaling. |

| Process | | | | | Outcomes | | | | |
|---|---|---|---|---|---|---|---|---|---|
| **Category** | **1 - Lagging** | **2 - Basic** | **3 - Intermediate** | **4 - Industry Leading** | **Category** | **1 - Lagging** | **2 - Basic** | **3 - Intermediate** | **4 - Industry Leading** |
| Impact Assessment<br><br>There is a process for evaluating the intended and unintended impacts of the AI system, including identifying who benefits and who is harmed. | The team has not evaluated who benefits and who harms from the AI system. | The team has evaluated some of the impacts of the AI system, both intended and unintended, and determined who benefits and who harms from the AI system. | The team has evaluated the most consequential and likely impacts of the AI system, both intended and unintended, and determined who benefits and who harms from the AI system. | The team has evaluated all the potential impacts of the AI system, both intended and unintended, and determined who benefits and who harms from the AI system. | Impact Assessment<br><br>Do the positive impacts of the AI system outweigh the negative? | The benefits of the AI system do not outweigh the harms. | The team has identified some potential harms and benefits, but there is not a full analysis.<br><br>Harms and benefits are described qualitatively.<br><br>Some mitigation strategies are listed, but are not comprehensive or tested. | There is some comparison that shows the benefits of the AI system outweigh the harms.<br><br>Some stakeholder groups and impacts are compared.<br><br>Some mitigation strategies are listed and piloted. | The team has conducted a full assessment that shows that the benefits outweigh the harms.<br><br>A structured framework was used for the assessment.<br><br>There are comprehensive and appropriate mitigations for any harms.<br><br>Monitoring plans are in place to detect unexpected outcomes. |
| Stakeholder Engagement<br><br>There is a process for engaging all relevant stakeholders, aligning with the RACI matrix, and incorporating feedback. | The team has not engaged any of the relevant stakeholders. | The team has engaged some of the relevant stakeholders and has incorporated some of their feedback. | The team has engaged most of the relevant stakeholders and has meaningfully incorporated most of their useful and valid input and feedback.<br><br>There are feedback mechanisms for most relevant stakeholders to provide their opinion on the value proposition and problem formulation surrounding the | The team has engaged representatives from all the stakeholder groups. Each stakeholder's involvement aligns with the RACI matrix column for value proposition and problem formulation.<br><br>There are easily accessible feedback mechanisms for all relevant stakeholders to provide their | Stakeholder Engagement<br><br>Has stakeholder input been taken into account? | The input from the relevant stakeholders has not been incorporated into the final testing and validation done. | Some of the input from the relevant stakeholders has not been incorporated into the final testing and validation done. | Most of the input from the relevant stakeholders has not been incorporated into the final testing and validation done. | All of the input from the relevant stakeholders has not been incorporated into the final testing and validation done in accordance with the ideal RACI matrix column for testing and validation. |

| Process | | | | | Outcomes | | | | |
|---|---|---|---|---|---|---|---|---|---|
| **Category** | **1 - Lagging** | **2 - Basic** | **3 - Intermediate** | **4 - Industry Leading** | **Category** | **1 - Lagging** | **2 - Basic** | **3 - Intermediate** | **4 - Industry Leading** |
| | | | AI system as the system moves through the subsequent stages of the lifecycle. | opinion on the value proposition and problem formulation surrounding the AI system as the system moves through the subsequent stages of the lifecycle. | | | | | |
| Process Documentation<br><br>There is a process for documenting decisions undertaken during this stage. | The team has not documented any of the processes taken in the testing and validation stage in a readily accessible manner. | The team has documented some of the processes taken in the testing and validation stage in a readily accessible manner. | The team has documented most of the processes taken in the testing and validation stage in a readily accessible manner. | The team has documented all of the processes taken in the testing and validation stage in a readily accessible manner. | Outcome Documentation<br><br>Have all the outcomes of this stage been documented? | The team has not documented any of the outcomes of the testing and validation stage in a readily accessible manner. | The team has documented some of the outcomes of the testing and validation stage in a readily accessible manner. | The team has documented most of the outcomes of the testing and validation stage in a readily accessible manner. | The team has documented all of the outcomes of the testing and validation stage in a readily accessible manner. |

# Deployment and Monitoring

| Process | | | | | Outcomes | | | | |
|---|---|---|---|---|---|---|---|---|---|
| **Category** | **1 - Lagging** | **2 - Basic** | **3 - Intermediate** | **4 - Industry Leading** | **Category** | **1 - Lagging** | **2 - Basic** | **3 - Intermediate** | **4 - Industry Leading** |
| End-user Guidance<br><br>There is a process for intentionally designing and communicating guidance for the end user to include who the system serves, for who/what it does not work, and understanding impacts of the end user decisions. | The team has not envisioned the experience of the end-user. | The team has envisioned the experience of the end-user to a limited extent and thought about some ways of providing guidance. | The team has envisioned the experience of the end-user and thought about ways of providing guidance.<br><br>The guidance includes some consideration of who the AI system works for and does not work for as determined in Testing and Validation.<br><br>The team has thought about whether the impacts of the decisions are understood by the end-user and whether the end-users will be making decisions that require their discretion / judgment. | The team has envisioned the experience of the end-user comprehensively and thought extensively about ways of providing guidance.<br><br>The guidance includes thorough consideration of who the AI system works for and does not work for as determined in Testing and Validation.<br><br>The team has thought about whether the impacts of the decisions are understood by the end-user and whether the end-users will be making decisions that require their discretion / judgment. | End-user Guidance<br><br>Is there good guidance for the end-user on how to use the AI system? | There is no guidance for the end-user on how to use the AI system. | There is limited guidance for the end-user on how to use the AI system.<br><br>Basic instructions may be provided for some features, but not all. Missing discussion of the potential impacts of decisions / judgement. | There is clear and structured guidance that covers main workflows and explains how to interpret outputs.<br><br>User manuals or help features describe some use cases. Documentation includes some possible impacts, but does not include edge cases or long term outcomes. | There is comprehensive guidance for the end-user on how to use the AI system.<br><br>The guidance includes a discussion on the impacts of the decisions and the discretion / judgment required by the end-users. |
| Use Case Guidance<br><br>Additional notes: this is more about what use | The team has not thought about the primary uses, secondary appropriate uses, or inappropriate | The team has thought about the primary uses, and inappropriate uses of the model. | The team has thought about the primary uses and inappropriate uses of the model, and has taken steps | The team has thought about the primary uses, secondary appropriate uses, and inappropriate uses of the | Use Case Guidance<br><br>Is there good guidance on the potential use cases of the AI system, and | There are inappropriate uses for the model, and no steps have been taken to prevent | There are inappropriate uses for the model, and some steps have been taken to prevent | The team has clearly defined primary use cases, and some inappropriate use cases have been identified. The team has | Thorough steps have been taken to prevent inappropriate use. These steps include steps for identifying / detecting |

| Process | | | | | Outcomes | | | | |
|---|---|---|---|---|---|---|---|---|---|
| **Category** | **1 - Lagging** | **2 - Basic** | **3 - Intermediate** | **4 - Industry Leading** | **Category** | **1 - Lagging** | **2 - Basic** | **3 - Intermediate** | **4 - Industry Leading** |
| cases the model is limited to.<br><br>There is a process for identifying primary and secondary use cases, as well as in/appropriate use cases, and communicating those to the end users. | uses of the model. | | (contractual and technical) to prevent inappropriate use and ensure that everyone who has access to the model is aware of potential inappropriate uses. | model, and has taken steps (contractual and technical) to prevent inappropriate use and ensure that everyone who has access to the model is aware of potential inappropriate uses. | which ones are appropriate / inappropriate? | inappropriate use.<br><br>False negatives or false positives create highly negative impacts for stakeholders. | inappropriate use.<br><br>Basic warnings or disclaimers highlight risky use cases. There is little enforcement ability or it is reactive.<br><br>False negatives or positives may only be partially mitigated. | begun to implement practical controls to mitigate inappropriate use.<br><br>Might include role based access, monitoring for common inappropriate use cases, etc. | inappropriate uses and checks / penalties to prevent inappropriate use.<br><br>False negatives or false positives do not create negative impacts for stakeholders, or appropriate and comprehensive mitigations have been planned. |
| System Transparency<br><br>There is a process for deciding the extent to which the methodology, datasets, code, and impact measurements can be publicized. | The team has not considered the extent to which the methodology, datasets, code, and impact measurements can be publicized.<br><br>In addition, no standard organizational defaults exist. | The team has not considered the extent to which the methodology, datasets, code, and impact measurements can be publicized.<br><br>Standard organizational defaults exist, but they are inadequate in some way (ex. Too broad, difficult to understand). | The team has not considered the extent to which the methodology, datasets, code, and impact measurements can be publicized, but adequate standard organizational defaults exist. | The team has considered the extent to which the methodology, datasets, code, and impact measurements can be publicized. | Open Access<br><br>Are the methodology / datasets / etc. publicized to the extent that is appropriate? | The methodology, datasets, code, and impact measurements are not publicized or shared with the relevant stakeholders even though it would be appropriate to be open about these components of the AI system. | The team has shared few of the methodology, datasets, code, and impact measurements , even if they are appropriate to be open about these components.<br><br>Basic documentation is accessible but datasets, code, or testing outcomes are not shared.<br><br>Access procedures are reactive or non existent. | The team has shared most of the methodology, datasets, code, and impact measurements , even if they are appropriate to be open about these components.<br><br>Datasets (anonymized if needed), scripts, performance measures are available in a controlled repository.<br><br>Access procedures (licensing, requests, etc) are available. | The methodology, datasets, code, and impact measurements are publicized to the extent to which it is appropriate to be open about these components of the AI system.<br><br>All of the non sensitive artifacts are available through clear procedures. |

| Process | | | | | Outcomes | | | | |
|---|---|---|---|---|---|---|---|---|---|
| **Category** | **1 - Lagging** | **2 - Basic** | **3 - Intermediate** | **4 - Industry Leading** | **Category** | **1 - Lagging** | **2 - Basic** | **3 - Intermediate** | **4 - Industry Leading** |
| Regulatory Compliance and Audits<br><br>There is a process for developing a regulatory and audit compliance plan. | The team has not considered the relevant regulatory requirements or a process for auditing their AI system. | The team has considered a few regulatory requirements or a process for auditing their AI system, but has not fully mapped these processes to the specific AI system. | The team has considered the relevant regulatory requirements or a process for auditing their AI system.<br><br>The process is broad. To actually execute the process, there would need to be further specification. | The team has considered the relevant regulatory requirements or a process for auditing their AI system.<br><br>The process is specific and detailed. To actually execute the process, there would not need to be further specification. | Regulatory Compliance<br><br>Does the AI system comply with regulatory standards? | The AI system does not meet relevant regulatory standards and there is no process for auditing the AI system. If the AI system has been audited, there is no audit trail. | The team has identified some key regulations, but compliance is partial at best.<br><br>An informal audit may have occurred, but no formal process or documentation exists. | The AI system meets most relevant regulatory standards and an audit process is in place.<br><br>There are compliance protocols with periodic reviews. Audit findings are documented.<br><br>There may still be some issues with the audit process (no details, missing signatures, no recommendation s for improvement). | The AI system meets relevant regulatory standards and there is a comprehensive process for auditing the AI system. If the AI system has been audited, there is a comprehensive audit trail, including the authority who audited the AI system and all recommendation s and decisions made. |
| Governance and Recourse<br><br>There is a process for providing recourse, explaining system decisions, and collecting deployment data. | The team has not considered a process for recourse for impacted community members, the privacy of the inference, or how to explain why a certain decision was made.<br><br>The team has not considered how and what data will be collected, and what will happen to this data. | The team has considered a process for recourse for impacted community members, the privacy of the inference, and how to explain why a certain decision was made.<br><br>The team has not considered how and what data will be collected, and what will happen to this data. | The team has considered a process for recourse for impacted community members, the privacy of the inference, and how to explain why a certain decision was made.<br><br>The process for recourse and explaining a decision is broad. To actually execute the process, there would need | The team has considered a process for recourse for impacted community members, the privacy of the inference, and how to explain why a certain decision was made.<br><br>The process for recourse and explaining a decision is specific and detailed. To actually execute the process, | Governance, and Audit Trails<br><br>Can the organization provide an explanation as to why any decision was made through the AI system? | There is no system for recourse for impacted community members.<br><br>The inference does not meet the appropriate privacy requirements.<br><br>There is no ability to provide an explanation as to why a certain decision was made. | Some mechanism exists for users to raise concerns, but it is not closely watched, or the public is not aware it is available.<br><br>Some safeguards and explanations exist for some outputs, but there are gaps. | A formal system is established and documented, but it may not be comprehensive.<br><br>Explanations exist for most decisions, includes confidence or other uncertainty/expla natory factors. | There is an easily accessible system for recourse for impacted community members.<br><br>The inference meets the appropriate privacy requirements.<br><br>For every decision, there is a comprehensive explanation as to why the decision was made. |

| Process | | | | | Outcomes | | | | |
|---|---|---|---|---|---|---|---|---|---|
| **Category** | **1 - Lagging** | **2 - Basic** | **3 - Intermediate** | **4 - Industry Leading** | **Category** | **1 - Lagging** | **2 - Basic** | **3 - Intermediate** | **4 - Industry Leading** |
| | | | to be further specification.<br><br>The team has considered how and what data will be collected, and what will happen to this data. | there would not need to be further specification.<br><br>The team has considered how and what data will be collected, and what will happen to this data. | | | | | The appropriate amount of data is being collected in an appropriate manner. The data is being dealt with in an appropriate manner. |
| Monitoring<br><br>There is a process for determining when data and model updates take place, observing interactions with the system, and detecting broader impacts over time. | The team has not thought about how the AI system will be monitored. | The team has thought about how the AI system will be monitored, but has failed to consider one or more critical aspects (ex. Ensuring ongoing data availability). | The team has thought about how the AI system will be monitored, considering all critical aspects such as ongoing data availability, data quality, data updating, model outputs, user interactions with the system, and broader impacts. | The team has thought about how the AI system will be monitored, considering all critical aspects such as ongoing data availability, data quality, data updating, model outputs, user interactions with the system, and broader impacts.<br><br>The team plans to conduct regular interviews with the users + impacted people as a part of the monitoring. | Monitoring<br><br>Is there good monitoring for the AI system? | There is not an implemented system for monitoring, including for continued data availability, data quality, and updating. | There is an implemented system for monitoring, including for continued data availability, data quality, or updating, but some aspects of the monitoring process are missing (ex. No plan for ensuring ongoing data availability) or the plans are not concrete (ex. No explicit plan for who will update the model and when). | There is a comprehensive monitoring system that tracks data availability, data quality, model outputs, etc.<br><br>Roles and responsibilities have been assigned, documented, and communicated.<br><br>User feedback channels may be under developed. | The monitoring system is implemented, technical tools exist and outputs are being used on a regular basis with alerts, for monitoring (data, model outputs, user interactions, and impact).<br><br>The team conducts regular interviews with the users + impacted people as a part of monitoring. |
| Maintenance and Updates<br><br>There is a process for determining the timing, | There is no guidance on when and how frequently data, model, and usage guidance updates should | There is guidance on the data, model, and usage guidance updates. | There is guidance on when and how frequently data, model, and usage guidance updates should | There is comprehensive guidance on when and how frequently data, model, and usage guidance | Maintenance and Updates<br><br>Is there good maintenance and are there regular | There are no data updates, model, updates, or usage guidance updates. Tests | Updates occur reactively or inconsistently, but there is no regular schedule. | There is a defined schedule and process for updates. Includes basic testing, | The data updates, model updates, and usage guidance updates are done on a regular basis |

| Process | | | | | Outcomes | | | | |
|---|---|---|---|---|---|---|---|---|---|
| **Category** | **1 - Lagging** | **2 - Basic** | **3 - Intermediate** | **4 - Industry Leading** | **Category** | **1 - Lagging** | **2 - Basic** | **3 - Intermediate** | **4 - Industry Leading** |
| frequency, of updates, as well as identifying who is responsible for testing and reviews. | be done, and who should be retesting and reviewing the AI system. | The guidance is very broad – it is missing key elements such as who should be retesting and reviewing the AI system, for example. | be done and who should be retesting and reviewing the AI system.<br><br>To actually follow the given guidance, there would need to be further specification. | updates should be done and who should be retesting and reviewing the AI system. | updates to the AI system? | are not run before rollout. | Some tests are run before updates, but there is no formal process or checklist.<br><br>Users may not be consistently notified of updates to user guidance. | preferably automated.<br><br>There are dedicated teams in place to review and validate updates before release.<br><br>User guidance is revised and communicated. | based on empirical evidence. Tests are run and reviewed by an assigned team before roll out.<br><br>User guidance is revised and communicated. |
| Risk Management, Harm Prevention, and Correction<br><br>Additional notes: this is more about what actions to take if there is harm occurring.<br><br>There is a process in place for evaluating the response team's plan across a variety of possible situations. | The team has not considered how to respond if the model causes harm, detect, or turn off / roll back the model if necessary. | The team has considered how to respond if the model causes harm.<br><br>The responses considered are limited – for example, the team has not considered turning off the model. | For the most impactful and likely situations, the team has considered how to respond.<br><br>The responses considered include turning off, rolling back, or overriding the model's decision. | The team has considered how to respond depending on a sufficient number of different possible situations.<br><br>The responses considered include turning off, rolling back, or overriding the model's decision. | Risk Management, Harm Prevention, and Correction<br><br>Is there a system for how to respond if the model causes harm, etc.? | There is no system for responding if the model causes harm, detecting and or turning off / rolling back the model. | The team has put basic safeguards in place, but lack a full response process.<br><br>A roll back procedure exists, but may not have been tested or roles assigned.<br><br>No automated detection processes. | The team has put a well defined monitoring and response plan in place with roles and processes.<br><br>There are automated monitoring and alert systems.<br><br>The roll back procedures exist and have been tested, and roles defined. | There is a comprehensive system for responding if the model causes harm or turning off / rolling back the model.<br><br>There are real time, automated monitoring and alert systems.<br><br>The roll back procedures exist and have been tested, and roles defined.<br><br>Reporting and audit logs capture incidents, decisions, and outcomes. |
| Stakeholder Engagement<br><br>There is a process for | The team has not engaged any of the relevant stakeholders. | The team has engaged some of the relevant stakeholders. | The team has engaged most of the relevant stakeholders and has meaningfully | The team has engaged representatives from all the stakeholder | Stakeholder Engagement | The input from the relevant stakeholders has not been | Some of the input from the relevant stakeholders has | Most of the input from the relevant stakeholders has been | All of the input from the relevant stakeholders has been |

| Process | | | | | Outcomes | | | | |
|---|---|---|---|---|---|---|---|---|---|
| **Category** | **1 - Lagging** | **2 - Basic** | **3 - Intermediate** | **4 - Industry Leading** | **Category** | **1 - Lagging** | **2 - Basic** | **3 - Intermediate** | **4 - Industry Leading** |
| engaging all relevant stakeholders, aligning with the RACI matrix, and incorporating feedback. | | | incorporated most of their useful and valid input and feedback.<br><br>There are feedback mechanisms for most relevant stakeholders to provide their opinion on the value proposition and problem formulation surrounding the AI system as the system moves through the subsequent stages of the lifecycle. | gorups. Each stakeholder's involvement aligns with the RACI matrix column for deployment and monitoring.<br><br>There are easily accessible feedback mechanisms for all relevant stakeholders to provide their opinion on the deployment and monitoring surrounding the AI system as the system moves through the subsequent stages of the lifecycle. | Has stakeholder input been taken into account? | incorporated into the deployment and monitoring. | been incorporated into the deployment and monitoring. | incorporated into the deployment and monitoring. | incorporated into the deployment and monitoring. in accordance with the ideal RACI matrix column for deployment and monitoring |
| Process Documentation<br><br>There is a process for documenting decisions undertaken during this stage. | The team has not documented any of the processes taken in the deployment and monitoring stage in a readily accessible manner. | The team has documented some of the processes taken in the deployment and monitoring stage in a readily accessible manner. | The team has documented most of the processes taken in the deployment and monitoring stage in a readily accessible manner. | The team has documented all of the processes taken in the deployment and monitoring stage in a readily accessible manner. | Outcome Documentation<br><br>Have all the outcomes of this stage been documented? | The team has not documented any of the outcomes of the deployment and monitoring stage in a readily accessible manner. | The team has documented some of the outcomes of the deployment and monitoring stage in a readily accessible manner. | The team has documented most of the outcomes of the deployment and monitoring stage in a readily accessible manner. | The team has documented all of the outcomes of the deployment and monitoring stage in a readily accessible manner. |
